# Supplementary material for: Can Large Language Models Assist the Comprehension of ROS2 Software Architectures?
Source: arXiv:2604.21699 source file (2026-04-23)
Supplement: Supplementary file 1 [file appendix.tex]

\onecolumn

\section{Computation Graphs and Distribution of Correct and Incorrect Answers}\label{s:pain}

\begin{figure}[h]
    \centering
    \includegraphics[width=0.5\linewidth]{vu-cs-research-thesis/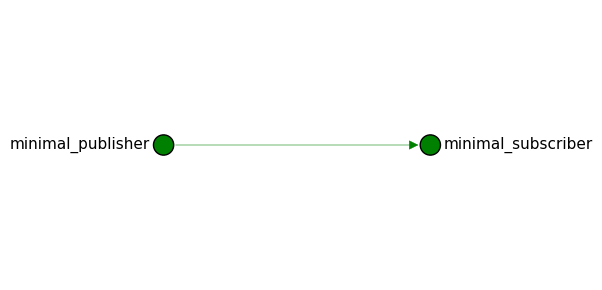}
    \caption{Coloured \texttt{\textbf{pubsub}} computation graph.}
    \label{fig:pubsub_pain}
\end{figure}

\begin{figure}[h]
    \centering
    \includegraphics[width=0.7\linewidth]{vu-cs-research-thesis/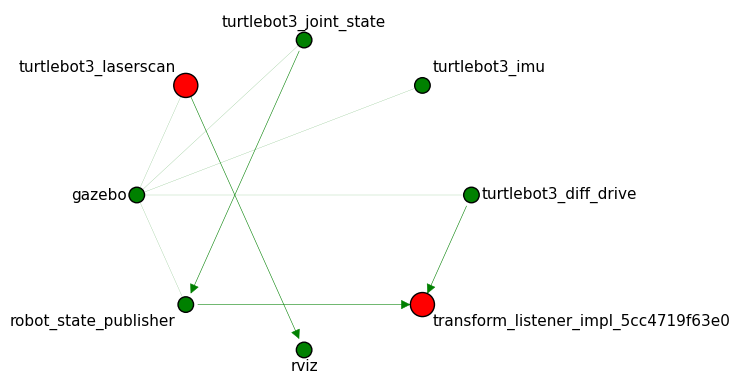}
    \caption{Coloured \texttt{\textbf{turtlebot}} computation graph.}
    \label{fig:turtlebot_pain}
\end{figure}

\begin{figure}[h]
    \centering
    \includegraphics[width=\linewidth]{vu-cs-research-thesis/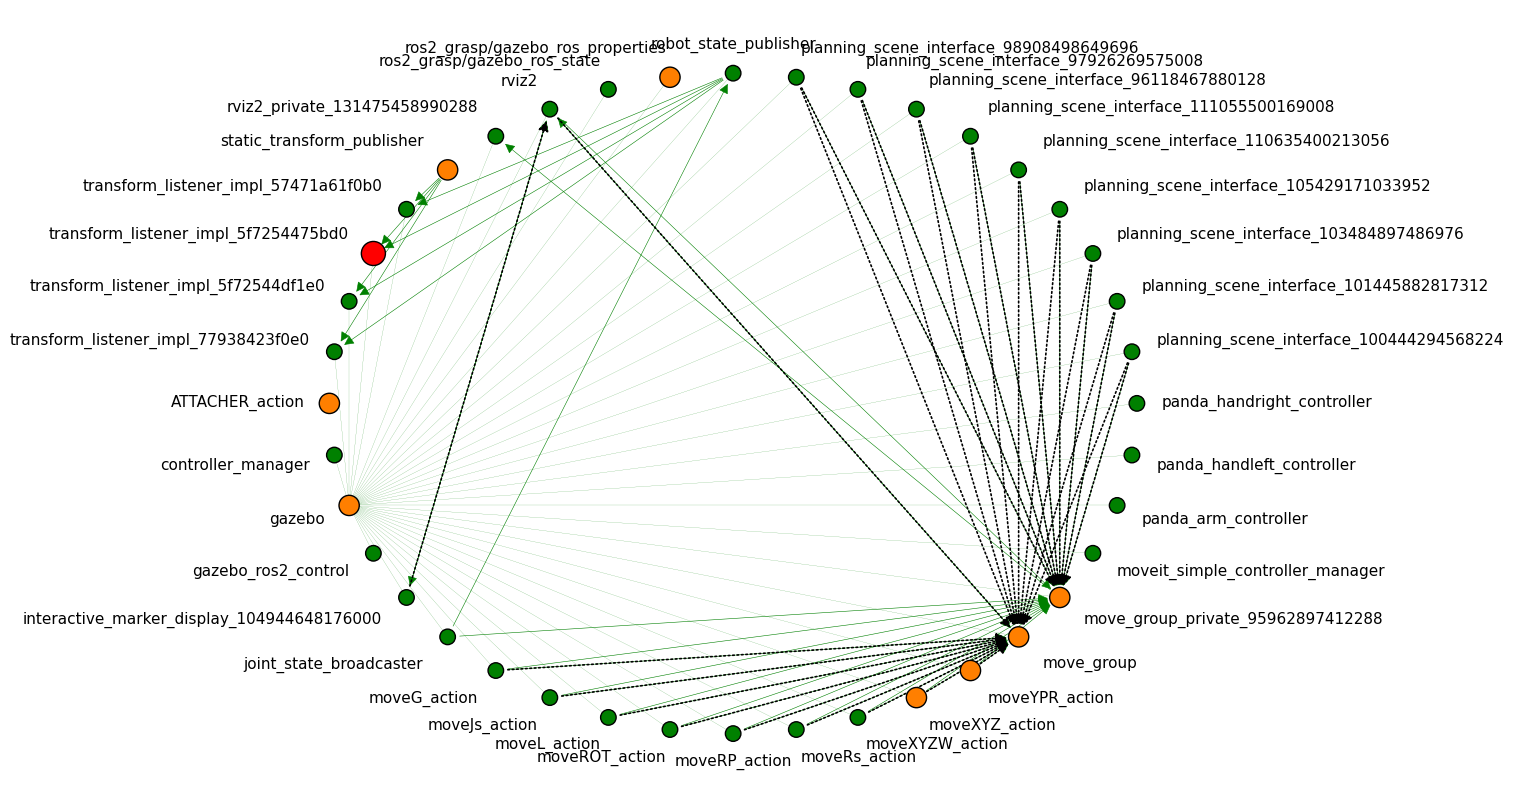}
    \caption{Coloured \texttt{\textbf{panda}} computation graph.}
    \label{fig:panda_pain}
\end{figure}

% \begin{figure}[H]
%   \centering
  
%   \begin{subfigure}{\linewidth}
%     \centering
%     \includegraphics[width=\linewidth]{vu-cs-research-thesis/figures/pubsub_graph.png}
%     \caption{Publisher–subscriber graph.}
%   \end{subfigure}

%   \begin{subfigure}{\linewidth}
%     \centering
%     \includegraphics[width=\linewidth]{vu-cs-research-thesis/figures/turtlebot_graph.png}
%     \caption{Turtlebot graph.}
%   \end{subfigure}

%   \begin{subfigure}{\linewidth}
%     \centering
%     \includegraphics[width=\linewidth]{vu-cs-research-thesis/figures/panda_graph.png}
%     \caption{Panda graph.}
%   \end{subfigure}

%   \caption{Comparison of different ROS 2 graphs.}
%   \label{fig:stacked_graphs}
% \end{figure}
